# Supplementary material for: Explicit formulas for the Variance of the State of a Linearized Power System driven by Gaussian stochastic disturbances
Source: arXiv:2302.06326 source file (2023-03-17)
Supplement: Supplementary file 1 [file syskuramotovar-supplement.tex]

% SIAM Supplemental File Template
\documentclass[review,supplement,onefignum,onetabnum]{siamart190516}

\input{ex-shared}

\externaldocument{syskuramoto-var}

% Optional PDF information
% \ifpdf
% \hypersetup{
%   pdftitle={Supplementary Materials: An Example Article},
%   pdfauthor={D. Doe, P. T. Frank, and J. E. Smith}
% }
% \fi

\begin{document}

\maketitle
TEXT

\end{document}
